# Supplementary material for: Sensitivity and specificity of a Bayesian single trial analysis for time varying neural signals
Source: arXiv:2001.11582 ancillary file (2020-01-30)
Supplement: Supplementary file 1 [file reviewer_responses.pdf]

## Reviews and Responses

**Publication Decision 1 from Neurons, Behavior, Data analysis, and Theory – October 4, 2019**

**Decision:** Revise and resubmit

### Comments from the editor:

Your manuscript has received its reviews. The reviewers ask for relatively minor changes, and I expect that I will be able to accept the paper conditioned on these changes happening.

However, I do agree with reviewer 2 that you should explore a larger range of the potential space of models. Such an additional analysis would make the paper more relevant for a broader range of scientists

### Response from the authors:

Thank you for handling our submission. We found the reviewer comments extremely positive and think that the suggestions resulted in an improved manuscript, which I have just submitted. I believe we have addressed all of the reviewer suggestions, and I've included a short response to each point below for extra clarification. Please pass along our thanks to the reviewers!

Note: Reviewer comments are italicized, author responses are in blue.

### Reviewer Comments

#### Reviewer #1:

*In this work, the authors investigate the performance of a Bayesian method for analysing spike count data. The method, introduced in a previous publication by the same group, is designed to distinguish between four alternative hypotheses on how neural activity encodes information about a pair of stimuli, which could be presented together or in isolation. These hypotheses include mechanisms such as winner-take-all (where the response to stimuli A and B together is equal to the response to either A or B in isolation, in a way that is constant or varying randomly across trials), summation or suppression (where  $AB > \max(A, B)$  or  $AB < \min(A, B)$ ), or averaging (where  $AB = wA + (1-w)B$  for some  $0 < w < 1$ ). Importantly, the method uses a single-trial approach, and can in principle differentiate between hypotheses that are undistinguishable with traditional, trial-averaged methods. In practical terms, the output of the method is a posterior probability over the four hypotheses it considers. To test its performance, the authors generate artificial spike count data according to one of the hypotheses, or according to rules representing simple deviations from one of them, and compare the posterior with the known ground truth. By analysing the results of these simulations, the authors show that their method performs well under reasonable conditions, similar to those that could be expected in a real-world scenario, and that it is robust to mild misspecification of the coding hypotheses.*

*This is a technical paper, addressing the performance of one specific method in a rather narrow use case. It could be seen as a companion paper to the authors' previous publication (Caruso et al, Nat Comm 2018). Therefore, the interest in the results presented here is likely to be limited in readers that are not already aware of the authors' other work. Nevertheless, the paper is overall internally consistent, the analyses are well explained and the results are convincing; it is also helpful to a potential reader that the scope of the work, and its strong relationship to Caruso et al 2018, is clearly signposted from the start. I recommend the paper for publication, with some suggestions for minor improvements that I outline below.*

- 1) *In the last paragraph of the main text, when discussing the importance of computational techniques that allow for single-trial analysis, it would be appropriate to cite some more recent work tackling this problem. In particular, I was reminded the literature on state-space models (see for instance Macke, Buesing and Sahani, "Estimating State and Parameters in State Space Models of Spike Trains" 2015 and Pandarinath et al 2018, doi:10.1038/s41592-018-0109-9).*

Regarding additional references to more recent single trial neural analyses, this was an excellent point and an oversight out our part. We have added some references to more recent work addressing similar questions.

- 2) *I enjoyed reading through the supplementary material; the authors have clearly made an effort to make the math accessible, to explain the reasoning behind their choices, and to explain the practical pitfalls of the numerical implementations wherever they arise. This is commendable. Some typos I spotted along the way:*
  - a. *on page 5, in the sentence that starts with "Therefore, to carry out": there is a stray "are" in the expression "...it is sufficient that we ARE evaluate..."*
  - b. *in the equation just below that, you are missing an integral sign after the first equality.*
  - c. *on page 6, towards the end: "This is because, the posterior distribution...": remove the comma.*

Thank you for noting these typos, which we have corrected in the new version of the supplement.

- 3) *Regarding reproducibility of the analysis and the availability of the code, I have tried to run the software made available by the authors and I have three observations:*
  - a. *remember that git does not version empty folders. So when someone clones your repo and runs the code according to the instructions in the master script, errors will be generated as the folders "data/" etc will not be found. This can be solved by adding a short README to these folders (maybe saying something like "This is the folder where generated data will go"), and adding that to the repo.*
  - b. *having the code available on github is great for accessibility, but please consider uploading the repo (or a just a tarball of a given version of the code) on a platform that will ensure a permanent record, such as Zenodo, before final publication.*
  - c. *in my own tests the code would run, but the default analysis described by the master script did not complete in a reasonable time (a few hours) on a recent laptop. It would be great if this could be changed to something that could be run in a shorter time, for a user that could be interested in testing whether the software runs on their machine.*

These were very useful suggestions for code accessibility, and we have implemented all of them. The default state of the code will also now run a much smaller subset of the analysis, so interested users can ensure it is working before committing to very long analysis runs.

#### **Reviewer #2:**

*This manuscript performs Bayesian analysis of single neuron spike trains from synthetic datasets. The authors aim to assess how the response of single neurons to the simultaneous presentation of two stimuli is related to single stimulus presentation. The manuscript is well written, and the idea presented is interesting, however, in the current status the results are pretty unconvincing and more work is required in order to make the manuscript appealing.*

*Their method works quite well in the example shown, however, only anecdotal evidence is presented so far. A systematic exploration of the high-dimensional parameter space is required.*

*First, results are not surprising given the high firing rates chosen for the simulations. The firing rate range used may be reasonable for higher order cortical areas in primates, but it is unrealistically large for rodents, given typical firing rates in mouse sensory cortex or hippocampus of about 1-5 Hz. The authors should repeat the same analysis within this more realistic firing rate range. Moreover, the authors should present a more thorough analysis of the accuracy of their inference in the two dimensional plane given by number of trials and mean evoked firing rate, for a fixed relative separation between the two A and B responses, as in the three panels of their Fig. 4. They should present phase boundaries in this trial-firing rate plane, to show where their method breaks down.*

The suggestion to include firing rates more relevant to rodent researchers was a welcome one, which we had not initially considered. In this revision, we extend the demonstration across a broader range of firing rates, and find that (as anticipated by the reviewer) very low firing rates prove difficult to categorize unless a large number of trials are analyzed. We think this additional analysis has strengthened the manuscript by providing a more complete, higher level picture of where and for what reasons the method begins to break down.

*How does the model scale with the number of stimuli presented? The authors should show what happens when more than 2 stimuli are present, each of which can elicit firing rate responses in an intermediate range.*

We agree with the reviewer that the question of how >2 stimuli might be handled is a very interesting one. Although it is outside the scope of the current analysis, we believe it to be a fruitful future direction for this research. Consequently, we have added a paragraph addressing this question to the discussion.
